# Supplementary material for: Learning Heatmap-Style Jigsaw Puzzles Provides Good Pretraining for 2D Human Pose Estimation
Source: arXiv:2012.07101 source file (2020-12-13)
Supplement: Supplementary file 1 [file supplementv1.pdf]

# Supplement Materials for Paper *Learning Heatmap-Style Jigsaw Puzzles Provides Good Pretraining for 2D Human Pose Estimation*

## 1. Human Keypoint Priors in Jigsaw Puzzles

We have mentioned in the article that there are positional priors for relative locations of human keypoints in person instances, which is an important reason why we consider solving self-supervised jigsaw puzzles as pretext task can provide efficient pretraining for 2D human pose estimation. In this section, we will elaborate on priors of human keypoints in jigsaw puzzles by statistical means.

### 1.1. Method for Statistical Analysis

In order to illustrate that the distributions of human keypoints have positional priors (i.e., some human keypoints are mainly distributed in certain image patches), we count the percentage of different image patches for each human keypoint in MSCOCO dataset [1]. To make our statistical results simple and easy for understanding, we take $N = 3$ as example for counting experiment in this section. Firstly, we divide each person instance in MSCOCO into three parts along both vertical and horizontal directions (i.e., $3 \times 3 = 9$ image patches in total), as Figure 1(a) in the main text demonstrates. Then, we calculate the probability that 17 different human keypoints falling within these $3 \times 3$ patches.

### 1.2. Statistical Results

MSCOCO keypoint annotations are with 17 human keypoints, 5 of which are annotated for the head (eyes, ears, nose), 6 are for upper limbs (shoulders, elbows, wrists), and 6 are for lower limbs (hips, knees, ankles). In order to make our statistical report clear, we note the 9 patches with their relative locations in person instances: *top-left, top, top-right, left, centre, right, bottom-left, bottom,* and *bottom-right*. According to statistical analyses, different human keypoints usually have their own priors of relative positions in person instances, and details for human keypoint priors are in the following part of this subsection..

(1) **Keypoint Priors for Head.** The analyses of head keypoint priors are demonstrated in Figure 1. Most of the head keypoints are located in the top parts of person instances (*top* takes the largest percentage, while *top-left/top-right* also count for some ratios). Based on this statistical result, we believe the following statement: if the network is able to distinguish whether each patch is in the top of the person instance in pretext task, the learnt features are also beneficial for predicting keypoints on the head.

(2) **Keypoint Priors for Lower Limbs.** The percentages of keypoints on lower limbs are shown in Figure 2. Similar to the distribution of head keypoints, the keypoints of lower limbs are also mainly distributed in several image patches, and the other patches count for only a small percentage in total. The hips are mainly near the centre of person instances, while knees and ankles are often near the bottom (i.e., *bottom, bottom-left, or bottom-right*) of person instances. Therefore, we consider that learning to classify centre patches in pretext task helps to locate hips in downstream human keypoint estimator, and learning the relative positions of bottom patches helps to locate knees and ankles.

(3) **Keypoint Priors for Upper Limbs.** Statistical priors for human keypoints on upper limbs are illustrated in Figure 3. Left/right shoulders are frequently located in the neighbourhoods of corresponding *top-left/top-right* patches. Apart from that, the *left/right* patches account for the largest percentages in the distributions of elbows/wrists, and their percentages are more than 10% higher than the second place. If the pretrained networks know how to distinguish the corresponding image patches in pretext task, it's helpful for localising keypoints on upper limbs in the downstream task.

### 1.3. Discussion for More Patches

We have expounded that different human keypoints have their own positional priors, and learning these priors by solving jigsaw puzzles problem is beneficial to the downstream pose estimator. We use $N = 3$ in this supplement material just to facilitate visualization and understanding. In practical experiments, $N$ can be any positive integer, and the position of each key point may be related to the priors of several image patches when $N$ is a larger number. The downstream 2D pose estimator performs best when $N = 6$.

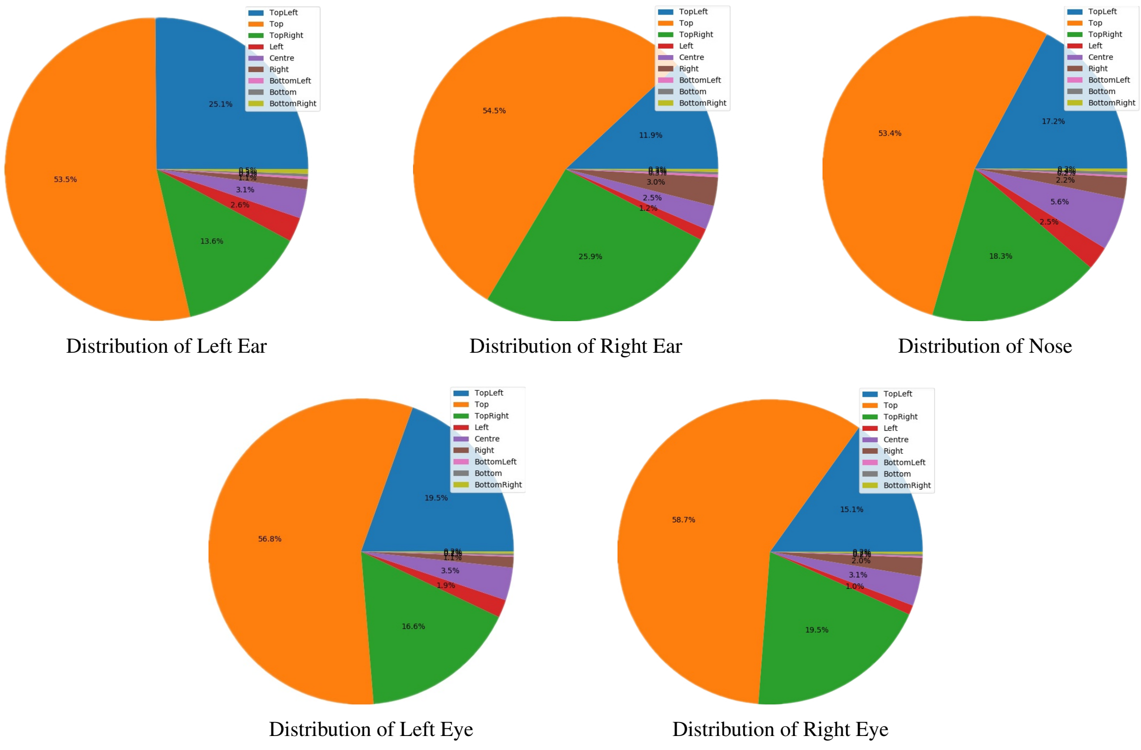


Figure 1: Positional analysis of head keypoints. Most of them are located in *top, top-left, or top-right* of person images.

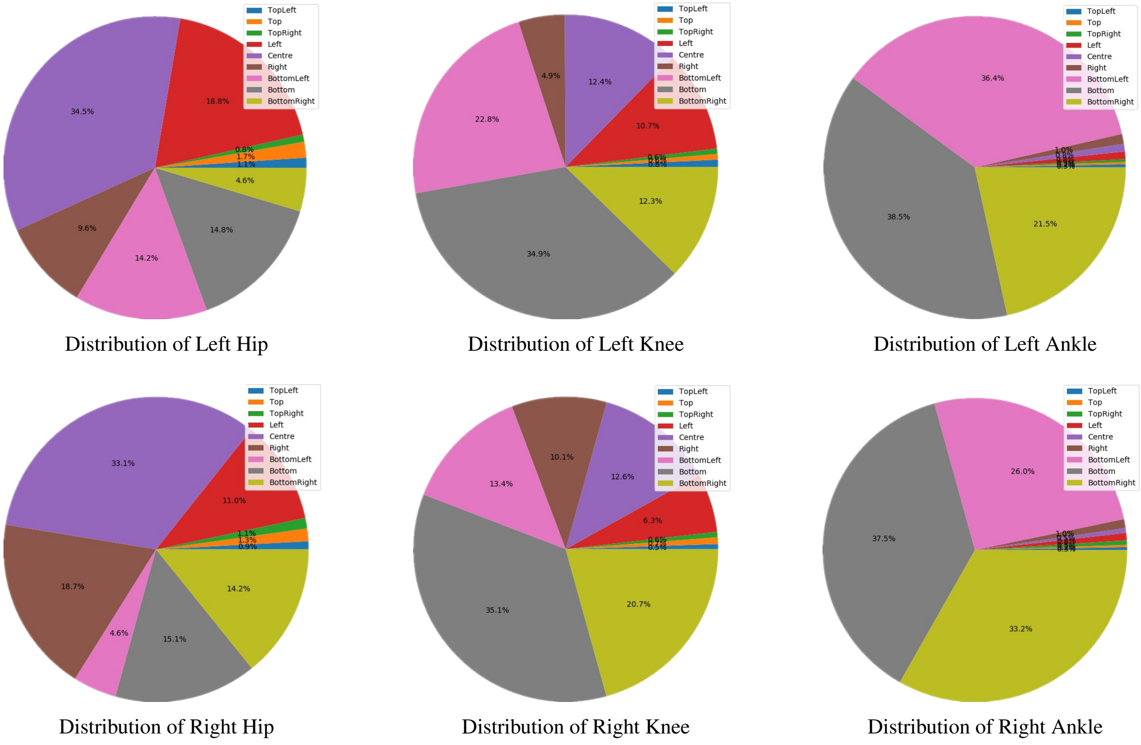


Figure 2: Positional analysis of human keypoints on lower limbs. Knees and Ankles are mainly located in bottom patches (*bottom, bottom-left, bottom-right*) of person instances, while hips are usually located in patches next to person centres.

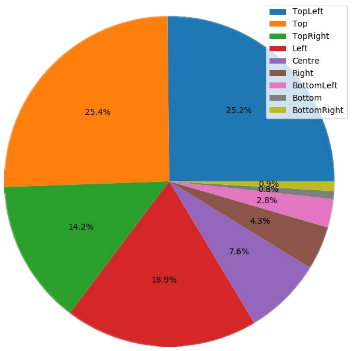


Distribution of Left Shoulder

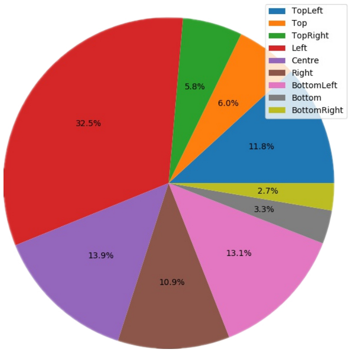


Distribution of Left Elbow

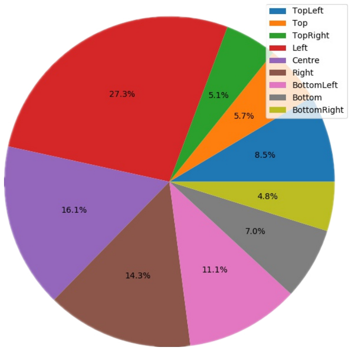


Distribution of Left Wrist

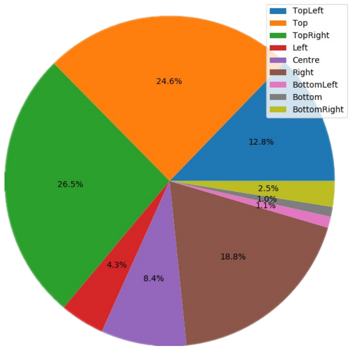


Distribution of Right Shoulder

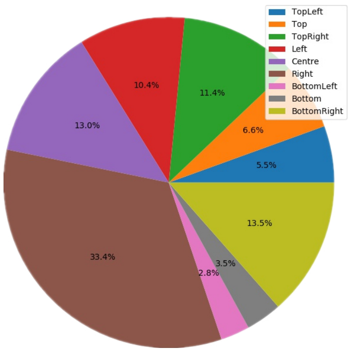


Distribution of Right Elbow

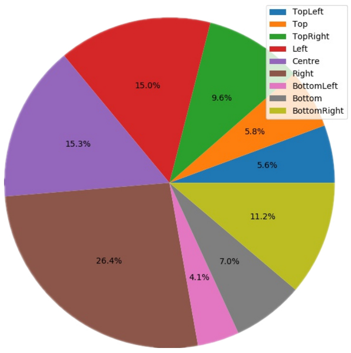


Distribution of Right Wrist

Figure 3: Positional analysis of human keypoints on upper limbs. Shoulders are usually next to top-left/top-right corners (i.e., *top, left/right, top-left/top-right*); *left/right* patches account for the largest percentage in elbow/wrist distributions.

## References

[1] Tsung-Yi Lin, Michael Maire, Serge J. Belongie, James Hays, Pietro Perona, Deva Ramanan, Piotr Dollár, and C. Lawrence Zitnick. Microsoft COCO: common objects in context. In *ECCV*, 2014. 1
